# Supplementary material for: 3DIAS: 3D Shape Reconstruction with Implicit Algebraic Surfaces
Source: arXiv:2108.08653 source file (2021-08-19)

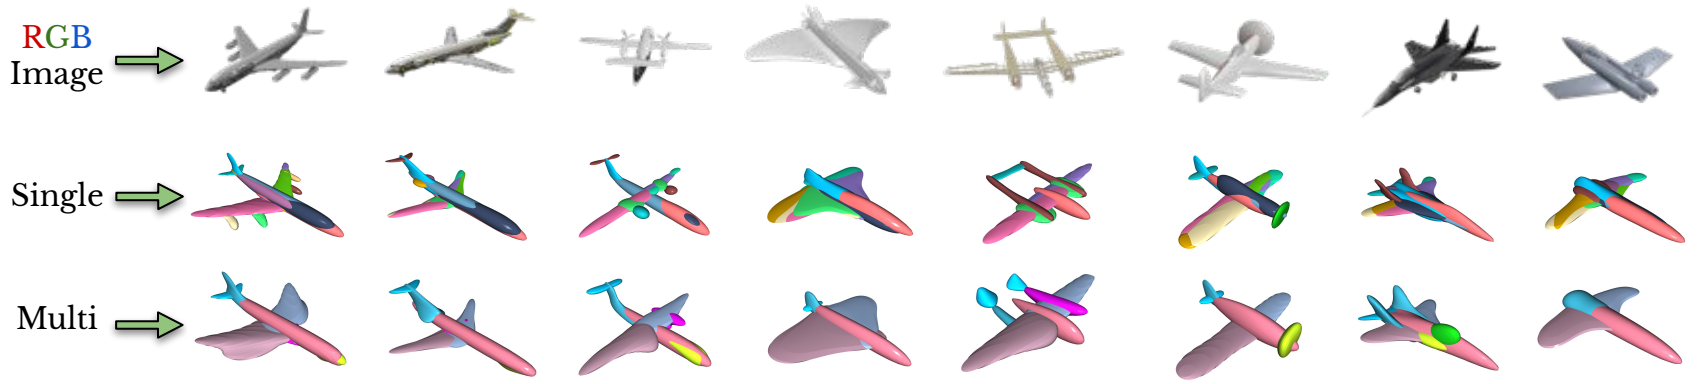

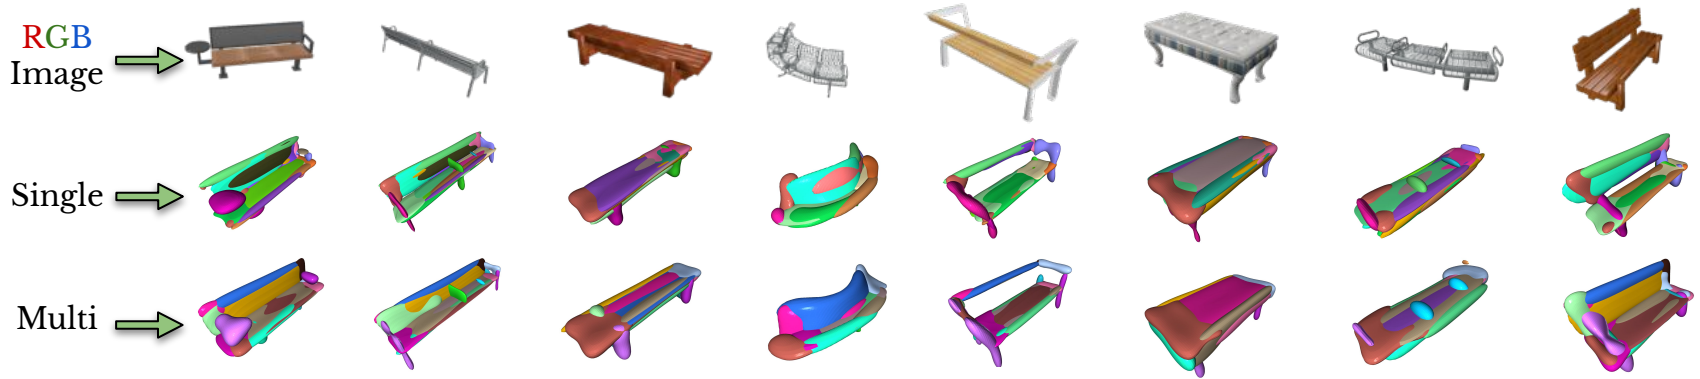

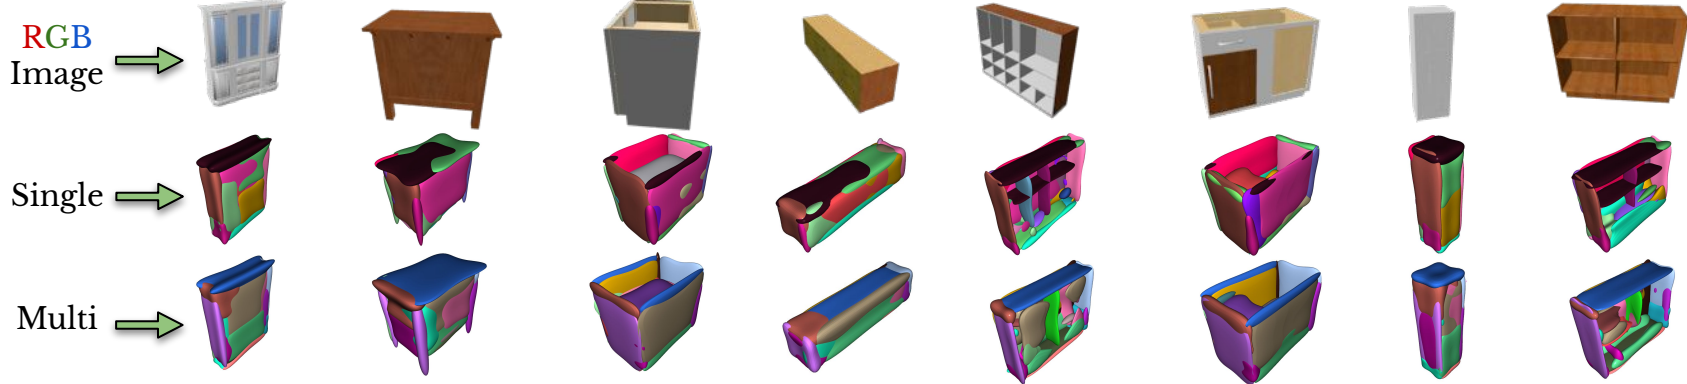

RGB  
Image

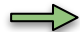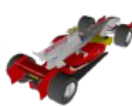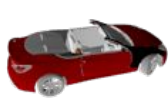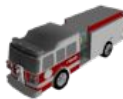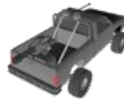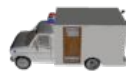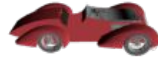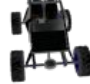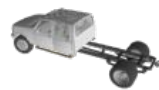

Single

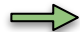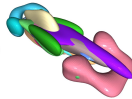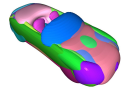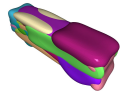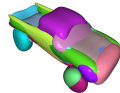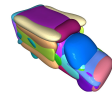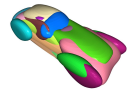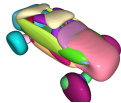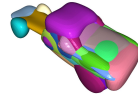

Multi

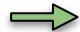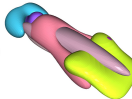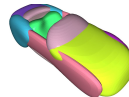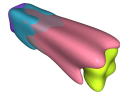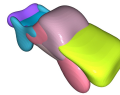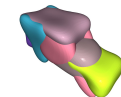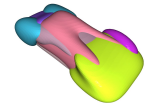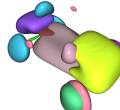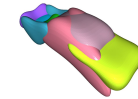



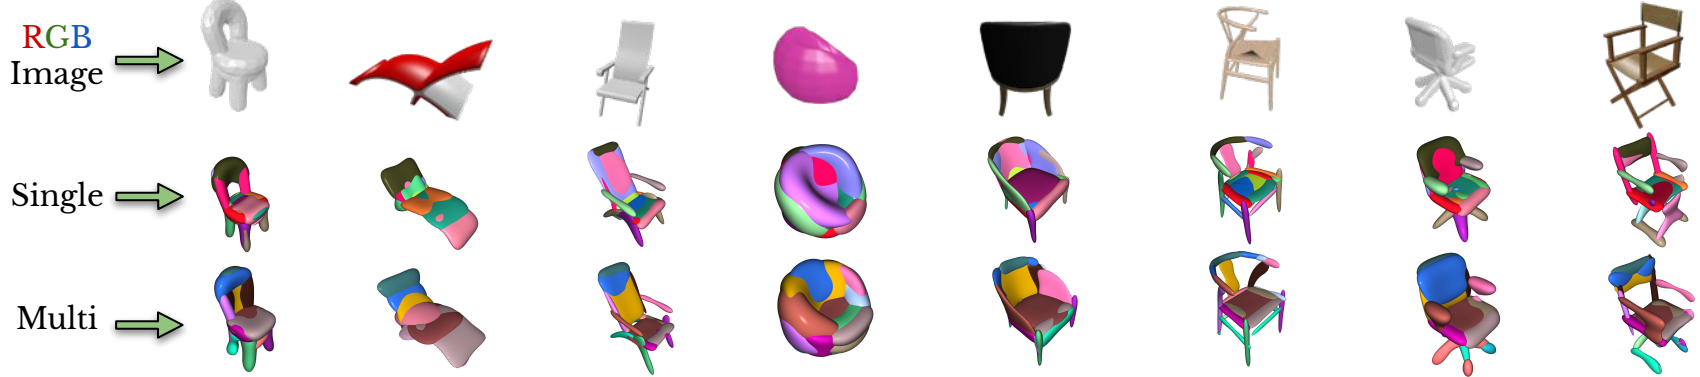

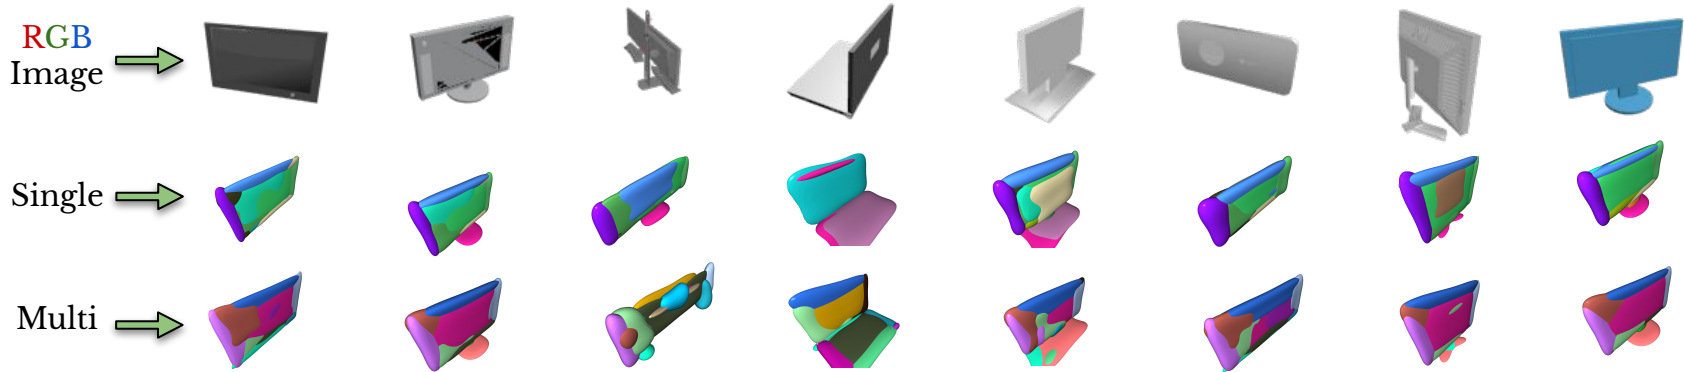

RGB  
Image

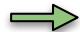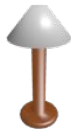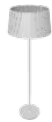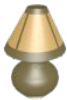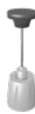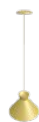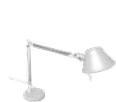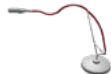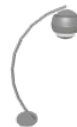

Single

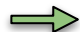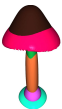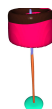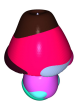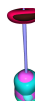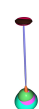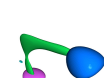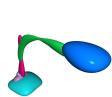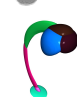

Multi

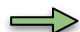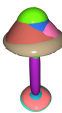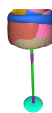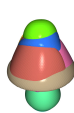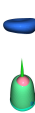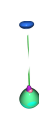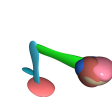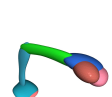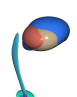

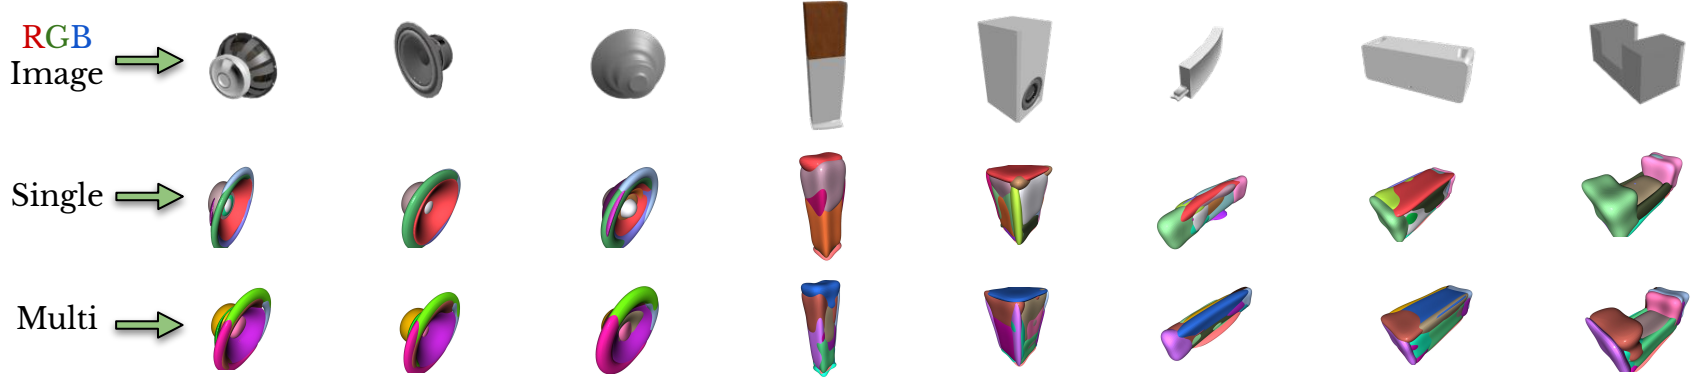

RGB  
Image

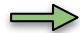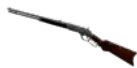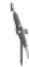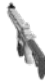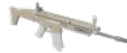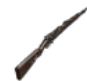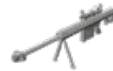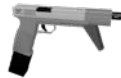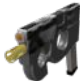

Single

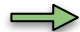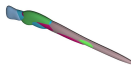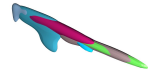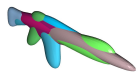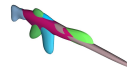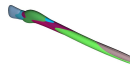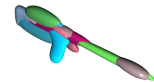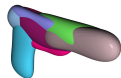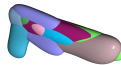

Multi

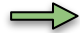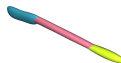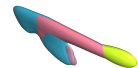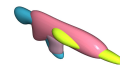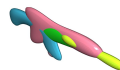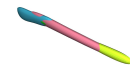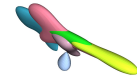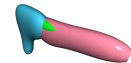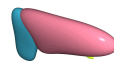

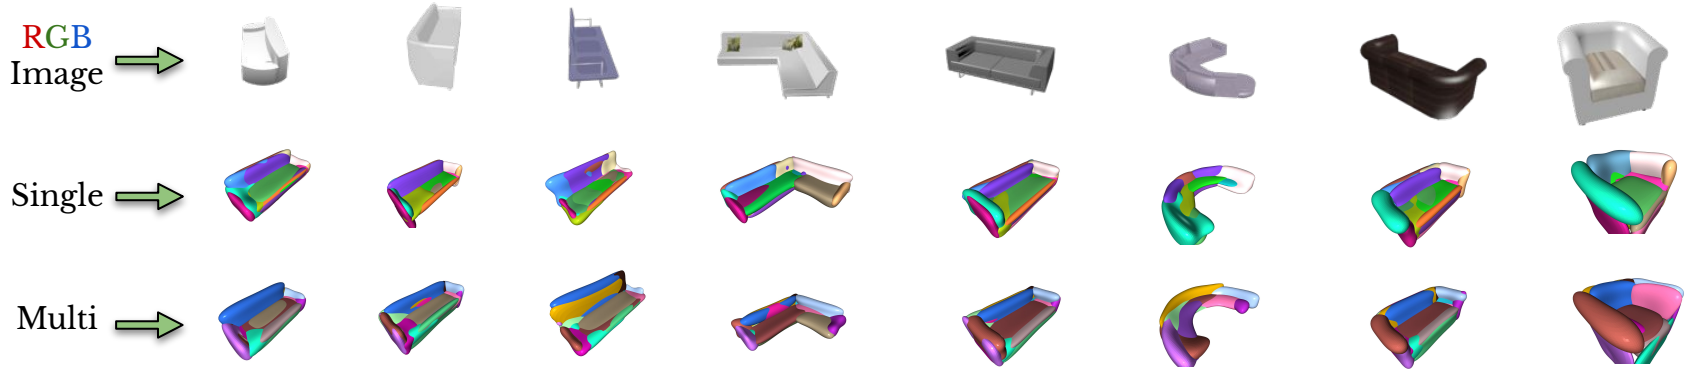

RGB  
Image

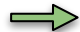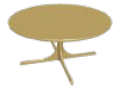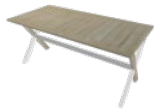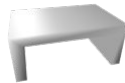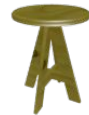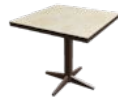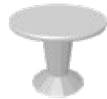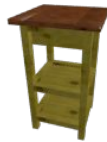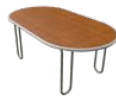

Single

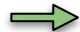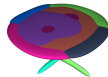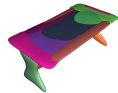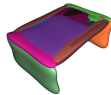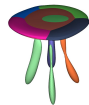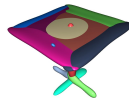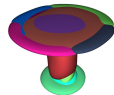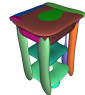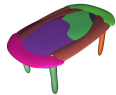

Multi

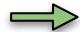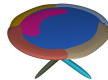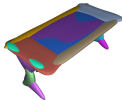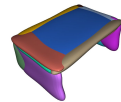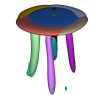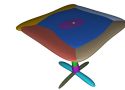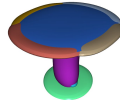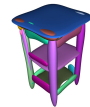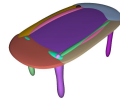

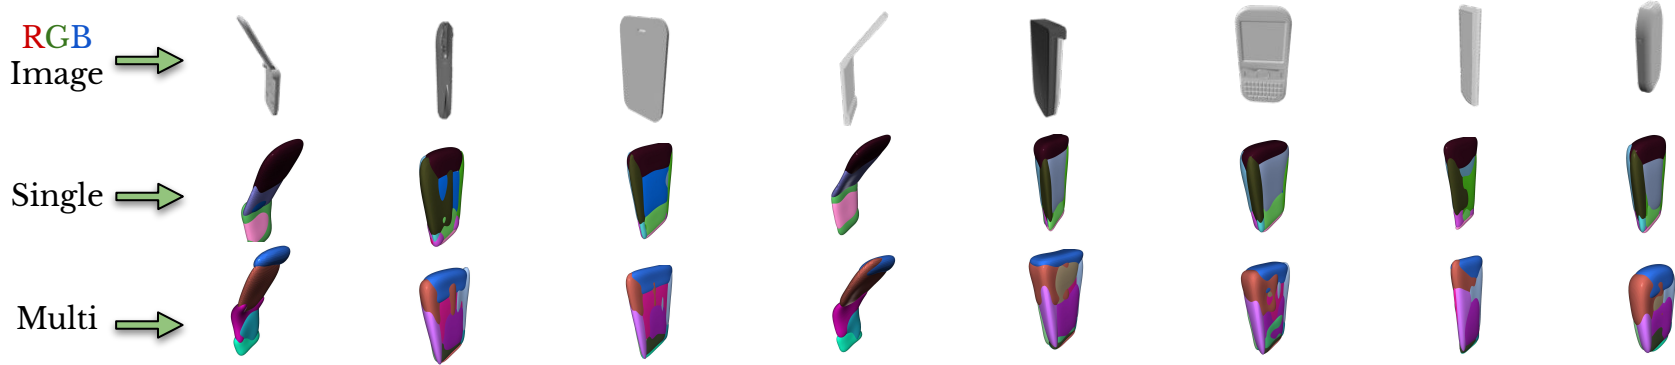



RGB  
Image

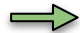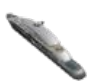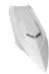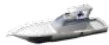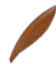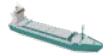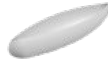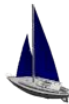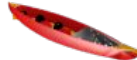

Single

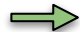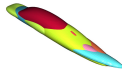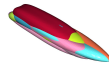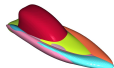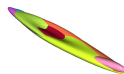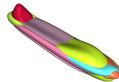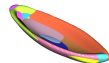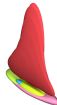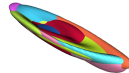

Multi

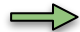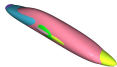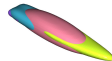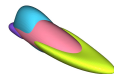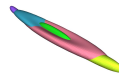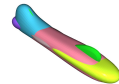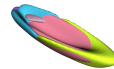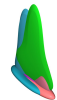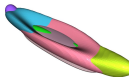

Supplement: Supplementary file 1 [file suppsinglemulti.pdf]
